# Supplementary material for: AttentionCode: Ultra-Reliable Feedback Codes for Short-Packet Communications
Source: arXiv:2205.14955 source file (2022-12-24)
Supplement: Supplementary file 1 [file AppendixB.tex]

\subsubsection{The self-attention block}
Considering a specific element in an input sequence, a self-attention block takes into account all other elements of the input sequence at the same time and decides which ones are more significant for the considered element by attributing different weights to other elements. The abstracted feature of the considered element is then the weighted sum of all the elements in the input sequence.

\begin{figure}
    \centering
    \includegraphics[width=0.55\columnwidth]{./figures/Fig_SelfAttention1.png}
    \caption{Illustration of the self-attention block.}
    \label{fig:SelfAttention1}
\end{figure}

An example is given in Fig.~\ref{fig:SelfAttention1}, where the input sequence is $[\bm{s_1,s_2,s_3,s_4,s_5}]$ and the output sequence (i.e., the abstracted features) is $[\bm{f_1,f_2,f_3,f_4,f_5}]$. Note that 1) each element of the input and output, i.e.,  $\bm{s_i}$ and $\bm{f_i}$, are both column vectors.
2) This example is only for illustration purposes to convey the main spirit. The detailed design of self-attention is more involved and can be found in our first progress report.

To compute $\bm{f_i}$, for example, there are two steps:
\begin{itemize}
\item Compute a score/correlation vector $[w_{1i},w_{2i},w_{3i},w_{4i},w_{5i}]^\top$, where
\begin{equation}
    w_{ji} = \bm{s_j}^\top \bm{s_i}.
\end{equation}
As can be seen, each entry in the score matrix is the inner product of two elements of the input sequence. Intuitively, it reflects how much we should attend to each input element when computing $\bm{f_i}$. It is worth noting that we often require the score vector to be a probability distribution. This can be realized by passing it through a softmax function.
\item Compute $\bm{f_i}$ by adding up the elements of the input sequence weighted by the score vector computed in the first step, giving
\begin{equation}
    \bm{f_i}=[\bm{s_1~s_2~s_3~s_4~s_5}]\times[w_{1i}~w_{2i}~w_{3i}~w_{4i}~w_{5i}]^\top.
\end{equation}
\end{itemize} 

\begin{figure}
    \centering
    \includegraphics[width=0.55\columnwidth]{./figures/Fig_SelfAttention2.png}
    \caption{Illustration of the self-attention block with a causal constraint.}
    \label{fig:SelfAttention2}
\end{figure}

\subsubsection{Causal mask}
When there is a causal constraint in the input sequence, $\bm{f_i}$ can only be computed based on $s_j$, $j\leq i$, but not $j>i$. In this context, we have to mask some of the entries in the score vector. As shown in Fig.~\ref{fig:SelfAttention2}, when computing $\bm{f_2}$, the last three entries of the score vector are masked to 0 so that $\bm{f_2}$  depends only on $\bm{s_1}$ and $\bm{s_2}$.
